# Supplementary material for: Hecke modifications of Higgs bundles and the extended Bogomolny equation
Source: arXiv:1812.08994 source file (2021-03-15)
Supplement: Supplementary file 1 [file Appendix.tex]

\section{Holomorphic principal $G^\C$--bundles and connections}

Let $\pi\co P^\C \to \Sigma$ be a principal $G^\C$--bundle.
Let $I$ be an $G^\C$--invariant complex structure with respect to which $\pi$ is holomorphic and
\begin{equation*}
  I (p\cdot \xi) = p\cdot i\xi,
\end{equation*}
that is, the $G^\C$--action is holomorphic as well.

Fix an arbitrary connection $A_0$.
With respect to the splitting
\begin{equation*}
  TP^\C \iso \pi^*TM\oplus P^\C\times \fg^\C
\end{equation*}
induced by $A_0$, we can write
\begin{equation*}
  I =
  \begin{pmatrix}
    I_\Sigma & 0 \\
    B_0 & i
  \end{pmatrix}
\end{equation*}
with $B_0 \in \pi^*TM \to \fg^\C$.
Since $I^2 = -\id$,
we have
\begin{equation*}
  iB_0 + B_0I_\Sigma = 0.
\end{equation*}
That is $a$ is complex anti-linear.

Let $a \in \Hom(\pi^*TM,\fg^\C)$ (understood with respect to $A_0$).
Consider the connection $A = A_0 + a$.
The relation between the splitting for $A_0$ and $A$ is given by the map
\begin{equation}
  (v,\xi) \mapsto (v,\xi-a(v))
\end{equation}
i.e.,
\begin{equation*}
  \begin{pmatrix}
    \one & 0 \\
    -a & \one
  \end{pmatrix}.
\end{equation*}
That is this map is the composition
\begin{equation*}
  T\Sigma\oplus\fg^\C \xrightarrow{A_0} TP \xrightarrow{A} T\Sigma\oplus\fg^\C.
\end{equation*}

The formula for $I$ in the decomposition for $A$ is
\begin{equation*}
  \begin{pmatrix}
    \one & 0 \\
    -a & \one
  \end{pmatrix}
  \begin{pmatrix}
    I_\Sigma & 0 \\
    B & i
  \end{pmatrix}
  \begin{pmatrix}
    \one & 0 \\
    a & \one
  \end{pmatrix}
  =
  \begin{pmatrix}
    I_\Sigma & 0 \\
    B_0 + ia - aI_\Sigma & i
  \end{pmatrix}.
\end{equation*}

This shows that the space of connection yielding the same $B$ is a torsor over $\Hom_\C(\pi^*TM,\fg^\C)$.
It also shows that we can always find a unique $a \in \overline{\Hom}_\C(\pi^*TM,\fg^\C)$ to cancel $B$.

%%% Local Variables:
%%% mode: latex
%%% TeX-master: "HeckeModificationsEBE"
%%% End:
